# Supplementary material for: Autonomous Learning for Face Recognition in the Wild via Ambient Wireless Cues
Source: arXiv:1908.09002 source file (2019-08-14)
Supplement: Supplementary file 1 [file appendix.tex]

%!TEX root = ../autotune.tex
\section{Appendix} % (fold)
\label{sec:appendix}

\subsection{Observations in Office and CommonRoom} % (fold)
\label{sub:observations_in_office_and_commonroom}
Fig.~\ref{fig:obs_oxford} and Fig.~\ref{fig:obs_tongji} show the attendance observations by WiFi sniffing and Cameras in the office and common room. Overall, both collected datasets have diverse group distribution and are very noisy. Automatically developing a face recognition system on them is challenging.

\begin{figure}[t!]
	\centering
	\begin{subfigure}{0.33\textwidth}
	\includegraphics[width=\linewidth]{fig/eval/oxford/camera_obs.pdf}
	\caption{Attendance observed by Camera}
	\end{subfigure}
	\hfill
	\begin{subfigure}{0.33\textwidth}
	\includegraphics[width=\linewidth]{fig/eval/oxford/wifi_obs.pdf}
	\caption{Attendance observed by WiFi} 
	\end{subfigure}
	\hfill
	\begin{subfigure}{0.33\textwidth}
	\includegraphics[width=\linewidth]{fig/eval/oxford/diff_obs.pdf}
	\caption{Attendance Noises} 
	\end{subfigure}
\caption{Attendance observations of 100 events in \emph{Office}. Three types of noises are highlighted with colors: errors of false-alarm devices (aka. face miss-capture) are in \emph{blue}; errors of false-alarm faces (aka. device miss-sniff) are in \emph{red}; non-POI disturbances are in \emph{orange}.} \label{fig:obs_oxford}
\end{figure}

\begin{figure}[t!]
	\centering
	\begin{subfigure}{0.98\textwidth}
	\includegraphics[width=\linewidth]{fig/eval/tongji/camera_obs.pdf}
	\caption{Attendance observed by Camera}
	\end{subfigure}
	\centering
	\begin{subfigure}{0.98\textwidth}
	\includegraphics[width=\linewidth]{fig/eval/tongji/wifi_obs.pdf}
	\caption{Attendance observed by WiFi} 
	\end{subfigure}
	\centering
	\begin{subfigure}{0.98\textwidth}
	\includegraphics[width=\linewidth]{fig/eval/tongji/diff_obs.pdf}
	\caption{Attendance Noises} 
	\end{subfigure}
\caption{Attendance observations of 100 events in \emph{CommonRoom}. Three types of noises are highlighted with colors: errors of false-alarm devices (aka. face miss-capture) are in \emph{blue}; errors of false-alarm faces (aka. device miss-sniff) are in \emph{red}; non-POI disturbances are in \emph{orange}.} \label{fig:obs_tongji}
\end{figure}

\subsection{More Face Identification Results} % (fold)
\label{sub:further_face_identification_results}
\subsubsection{Results on Office Dataset} % (fold)
\label{ssub:results_on_office_dataset}

% subsubsection results_on_office_dataset (end)
We provide the confusion matrix of the rank-1 prediction of AutoTune and competing approaches on two real-world datasets. Details of this experiment can found in \sect\ref{ssub:face_identification}. We note that rank-1 predictions of subject $\#3$ on the office dataset is very inaccurate with $0\%$ accuracy. By inspecting the source data, we observed that the low accuracy is because the errors of false-alarm devices of this subject are significant. As a result, the true image cluster of subject $\#3$ is not very compatible with her device based on the event vectors. It turns out that her device ID is more similar to another subject's ($\#15$) image clusters, which possess those ``missed'' event attendance information. Moreover, we also observed that both subject $\#3$ and $\#5$ are female with the same ethnicity, and the pre-trained model finds itself difficult to differentiate their faces as well. Therefore, AutoTune fails to label her images due to both insufficient face discrimination given by the pre-trained model (i.e., bad initialization) and non-informative device observations.

Note that, as discussed in \sect\ref{ssub:voting}, we always set a greater number of clusters than the number of POI in clustering, to help deal with the uncertain presences of non-POI. Therefore, although one image cluster of subject $\#15$ is mis-associated with the label $\#3$, it does not affect the recognition performance of subject $\#15$, as there is another image cluster of subject $\#15$, which matches her device's presence pattern more, and is labeled correctly. We here highlight that this robustness is brought by the voting capability.

Although AutoTune fails to predict subject $\#3$, it still has the best overall accuracy compared to other competing approaches. AutoTune's Cumulative Match Characteristic of identification is also shown to be the best among all the methods (see \sect\ref{ssub:face_identification}).
\begin{figure}[h!]
	\centering
	\begin{subfigure}{0.48\textwidth}
	\includegraphics[width=\linewidth]{fig/eval/oxford/cm_oxford_TM.pdf}
	\caption{TM} 
	\end{subfigure}\hspace*{\fill}
	\begin{subfigure}{0.48\textwidth}
	\includegraphics[width=\linewidth]{fig/eval/oxford/cm_oxford_OA.pdf}
	\caption{OA}
	\end{subfigure}
	\medskip
	\centering
	\begin{subfigure}{0.48\textwidth}
	\includegraphics[width=\linewidth]{fig/eval/oxford/cm_oxford_DT.pdf}
	\caption{D-AutoTune} 
	\end{subfigure}\hspace*{\fill}
	\begin{subfigure}{0.48\textwidth}
	\includegraphics[width=\linewidth]{fig/eval/oxford/cm_oxford_AutoTune.pdf}
	\caption{AutoTune} \label{fig:cm_ox}
	\end{subfigure}
\caption{Confusion matrix of face identification with 20 people using different methods on the \emph{office} dataset.}
\end{figure}

\subsubsection{Results on CommonRoom Dataset} % (fold)
\label{ssub:results_on_commonroom_dataset}
The results on the CommonRoom dataset is much neater and the rank-1 prediction of AutoTune is superior to the competing approaches. However, we note that there are $\sim 29\%$ predictions of the subject $\#7$ that are mis-classified to subject $\#4$. By looking into the source data, we found that the number of his face images is too limited in the training data, due to lack of event participation. This limited dataset does not contain many variations that can enable his learnt face features.

\begin{figure}[h!]
	\centering
	\begin{subfigure}{0.48\textwidth}
	\includegraphics[width=\linewidth]{fig/eval/tongji/cm_tongji_TM.pdf}
	\caption{TM} 
	\end{subfigure}\hspace*{\fill}
	\begin{subfigure}{0.48\textwidth}
	\includegraphics[width=\linewidth]{fig/eval/tongji/cm_tongji_OA.pdf}
	\caption{OA}
	\end{subfigure}
	\medskip
	\centering
	\begin{subfigure}{0.48\textwidth}
	\includegraphics[width=\linewidth]{fig/eval/tongji/cm_tongji_DT.pdf}
	\caption{D-AutoTune} 
	\end{subfigure}\hspace*{\fill}
	\begin{subfigure}{0.48\textwidth}
	\includegraphics[width=\linewidth]{fig/eval/tongji/cm_tongji_AutoTune.pdf}
	\caption{AutoTune}
	\end{subfigure}

\caption{Confusion matrix of face identification with $12$ people using different methods on the \emph{CommonRoom} dataset.}
\end{figure}
% section further_results_of_online_face_identification (end)
